# Supplementary material for: UIBDiffusion: Universal Imperceptible Backdoor Attack for Diffusion Models
Source: arXiv:2412.11441 source file (2025-02-28)
Supplement: Supplementary file 1 [file supplementary.tex]

\subsection{Why choose UAP for Diffusion}
Theoretical Analysis of UAP Escaping Elijah's Removal

\paragraph{Pre-Conditions}

\subsubsection{Definitions and Variable Relationships}
\begin{definition}[Key Variables and Their Relationships]
The following variables and their relationships are fundamental to our analysis:
\begin{enumerate}
\item $\lambda_t$: The scale of distribution shift at timestep $t$:
    \begin{equation}
        \lambda_t = \frac{\|M_\theta(x_t + \delta^*) - M_\theta(x_t)\|}{\|\delta^*\|} = \frac{c_t}{\sqrt{\bar{\alpha}_t}}
    \end{equation}
\item $\tau$: The inverted trigger pattern identified by Elijah's detection mechanism
\item $threshold_{shift}$: Maximum allowable distribution shift:
    \begin{equation}
        threshold_{shift} = \frac{\epsilon_{detect}}{L}
    \end{equation}
\item Model constants:
    \begin{itemize}
        \item $L = \prod_{i=1}^n \|W_i\|$ (Lipschitz constant)
        \item $\beta = \frac{L^2}{2\min_{x}\sigma_{min}(H(x))}$ (Second-order coefficient)
        \item $c_t = \frac{1-\bar{\alpha}_t}{\bar{\alpha}_t}$ (Diffusion schedule coefficient)
    \end{itemize}
\end{enumerate}
These variables satisfy the following relationships:
\begin{equation}
    \|\tau\| \geq \frac{\text{dist}(f(x), y_t)}{L} \gg \|\delta^*\|
\end{equation}
\end{definition}
\subsubsection{Understanding Elijah's Original Mechanism}
To accurately analyze how UAP evades detection, we first need to understand Elijah's original backdoor removal mechanism. Elijah identifies and removes backdoor functions through:
\begin{equation}
f_{\text{clean}}(x) = f(x) - \sum_{i=1}^K w_i \cdot f_i(x)
\end{equation}
where $f_i(x)$ represents identified backdoor functions, and the weights $w_i$ are optimized via:
\begin{equation}
w^* = \arg\min_w \mathbb{E}{(x,y)\sim\mathcal{D}{\text{clean}}}[\mathcal{L}(f_{\text{clean}}(x), y)]
\end{equation}
\subsubsection{Bridging Elijah's Method and Distribution Shift}
We extend Elijah's framework by showing how the backdoor function $f_i(x)$ manifests as a distribution shift:
\begin{theorem}[Backdoor Function Decomposition]
For a UAP-based backdoor $\delta^$, the backdoor function $f_i(x)$ can be decomposed as:
\begin{equation}
f_i(x) = M_\theta(x + \delta^) - M_\theta(x) = \Delta_{shift}(x) + \Delta_{noise}(x)
\end{equation}
where $\Delta_{shift}(x)$ represents the systematic distribution shift and $\Delta_{noise}(x)$ captures model non-linearity effects.
\end{theorem}
% \begin{proof}[Proof of Backdoor Function Decomposition]
% Given a UAP-based backdoor $\delta^*$, we can decompose $f_i(x)$ via Taylor expansion:
% \begin{equation}
%     f_i(x) = M_\theta(x + \delta^*) - M_\theta(x) = \nabla_xM_\theta(x)\delta^* + \frac{1}{2}\delta^{*T}H(x)\delta^*
% \end{equation}
% where:
% \begin{itemize}
%     \item $\Delta_{shift}(x) = \nabla_xM_\theta(x)\delta^*$ represents the first-order linear shift
%     \item $\Delta_{noise}(x) = \frac{1}{2}\delta^{*T}H(x)\delta^*$ captures the second-order non-linear effects
%     \item $H(x)$ is the Hessian matrix
% \end{itemize}
% This decomposition is justified by the model's differentiability and local behavior.
% \end{proof}

\begin{proof}[Proof of Backdoor Function Decomposition]
Given a twice differentiable model $M_\theta$, by Taylor's theorem [cite: Taylor expansion theorem], we have:
\begin{equation}
    f_i(x) = M_\theta(x + \delta^*) - M_\theta(x) = \nabla_xM_\theta(x)\delta^* + \frac{1}{2}\delta^{*T}H(x)\delta^* + R(\delta^*)
\end{equation}
where $R(\delta^*)$ is the remainder term with $\|R(\delta^*)\| = o(\|\delta^*\|^2)$.

The remainder term $R(\delta^*)$ satisfies $\|R(\delta^*)\| = o(\|\delta^*\|^2)$ under the following conditions:
\begin{enumerate}
    \item $M_\theta$ has bounded third derivatives: $\|\nabla^3 M_\theta(x)\| \leq K$ for some K
    \item The perturbation satisfies $\|\delta^*\| \leq \min\{1, \frac{1}{K}\}$
    \item For any $\xi \in [0,1]$:
    \begin{equation}
        \|\nabla^3 M_\theta(x + \xi\delta^*)\| \leq K
    \end{equation}
\end{enumerate}

Therefore:
\begin{equation}
    \Delta_{shift}(x) = \nabla_xM_\theta(x)\delta^* 
\end{equation}
\begin{equation}
    \Delta_{noise}(x) = \frac{1}{2}\delta^{*T}H(x)\delta^* + R(\delta^*)
\end{equation}
\end{proof}
\paragraph{UAP Shift}

\subsubsection{Problem Formulation and Preliminaries}
Given a diffusion model $M_{\theta}$ and a Universal Adversarial Perturbation (UAP) $\delta^*$, we analyze why UAP-based backdoor triggers can escape Elijah's removal mechanism. We first formalize the key components:
\begin{definition}[Distribution Shift Detection]
Through the backdoor function decomposition, we can measure the distribution shift between clean and triggered inputs:
\begin{equation}
Loss_{rb} = \mathbb{E}t[\mathbb{E}{x_t^c}[|M_\theta(x_t^c + \lambda_t\tau) - M_\theta(x_t^c)|]]
\end{equation}
where $\tau$ is the inverted trigger and $\lambda_t$ is the shift coefficient at timestep $t$.
\end{definition}
\subsubsection{UAP's Small Distribution Shift Property}
The key insight lies in UAP's optimization objective:
\begin{theorem}[UAP Minimal Shift]
A well-designed UAP $\delta^$ satisfies:
\begin{equation}
\delta^ = \arg\min_\delta {|\delta|p : \mathbb{P}{x\sim\mathcal{D}}[f(x+\delta) \neq f(x)] \geq \theta}
\end{equation}
where $\theta$ is the target success rate.
\end{theorem}
This leads to two crucial properties:
\begin{lemma}[Distribution Movement Minimality]
The expected distribution shift induced by UAP is bounded:
\begin{equation}
|\mathbb{E}{x\sim N(\mu,\sigma^2)}[x+\delta^*] - \mathbb{E}{x\sim N(\mu,\sigma^2)}[x]| = |\delta^*| \ll |\tau|
\end{equation}
\end{lemma}

\begin{proof}[Complete Proof of Distribution Movement Minimality]
Let's prove this step by step:

1) By definition of UAP optimization:
\begin{equation}
    \|\delta^*\| = \min\{\|\delta\|: \mathbb{P}[f(x+\delta) \neq f(x)] \geq \theta\}
\end{equation}

2) For traditional trigger $\tau$:
\begin{equation}
    \|\tau\| \geq \min\{\|\delta\|: f(x+\delta) = y_t\}
\end{equation}

3) Given $\mathcal{S}_1 = \{\delta: f(x+\delta) = y_t\}$ and $\mathcal{S}_2 = \{\delta: f(x+\delta) \neq f(x)\}$:
\begin{equation}
    \mathcal{S}_1 \subset \mathcal{S}_2
\end{equation}

4) Therefore:
\begin{equation}
    \min_{\delta \in \mathcal{S}_2} \|\delta\| \leq \min_{\delta \in \mathcal{S}_1} \|\delta\|
\end{equation}

5) To justify $\|\delta^*\| \ll \|\tau\|$, we need to show:
\begin{itemize}
    \item For any misclassification $f(x+\delta) \neq f(x)$, the required perturbation magnitude is:
    \begin{equation}
        \|\delta_{misc}\| \approx \frac{\text{margin}(f,x)}{\|\nabla f(x)\|}
    \end{equation}
    where $\text{margin}(f,x)$ is the distance to decision boundary
    
    \item For targeted attack $f(x+\delta) = y_t$, the required magnitude is:
    \begin{equation}
        \|\delta_{target}\| \geq \frac{\text{dist}(f(x), y_t)}{\|\nabla f(x)\|}
    \end{equation}
    
    \item By definition of classification margins:
    \begin{equation}
        \text{margin}(f,x) \ll \text{dist}(f(x), y_t)
    \end{equation}
\end{itemize}

Therefore, $\|\delta^*\| \ll \|\tau\|$ holds under these conditions.
\end{proof}

6) The expected distribution shift follows directly:
\begin{equation}
    \|\mathbb{E}_{x\sim N(\mu,\sigma^2)}[x+\delta^*] - \mathbb{E}_{x\sim N(\mu,\sigma^2)}[x]\| = \|\delta^*\| \ll \|\tau\|
\end{equation}

\begin{proof}
Given UAP $\delta^*$ and traditional trigger $\tau$:
\subsection{Escape Mechanism Analysis}
When using UAP as a trigger, we can establish:
\begin{proposition}[Distribution Shift Threshold]
The distribution shift $\lambda_t$ induced by UAP satisfies:
\begin{equation}
\lambda_t|\delta^*| < threshold_{shift}
\end{equation}
where $threshold_{shift}$ is Elijah's removal threshold.
\end{proposition}
Considering Elijah's complete removal loss:
\begin{equation}
Loss_\theta = Loss_{rb} + Loss_{mc} + Loss_{dm}
\end{equation}
We can prove:
\begin{theorem}[UAP Escape Condition]
When $\lambda_t|\delta^|$ is sufficiently small:
\begin{equation}
|\mathbb{E}{\epsilon}[M\theta(\epsilon + \delta^) - M_\theta(\epsilon)]| < \epsilon_{detect}
\end{equation}
where $\epsilon_{detect}$ is the detection threshold, the UAP-based backdoor can escape detection.
\end{theorem}
This leads to three key implications:
\begin{corollary}[Removal Ineffectiveness]
\begin{enumerate}
\item The removal loss cannot effectively identify and penalize small distribution shifts
\item The model preserves the original distribution rather than removing the backdoor
\item Clean accuracy is maintained while backdoor effectiveness persists
\end{enumerate}
\end{corollary}
From UAP optimization:
\begin{equation}
|\delta^*| = \min{|\delta|: \mathbb{P}[f(x+\delta) \neq f(x)] \geq \theta}
\end{equation}
For any effective trigger $\tau$:
\begin{equation}
|\tau| \geq \min{|\delta|: f(x+\delta) = y_t}
\end{equation}
Since UAP seeks minimal perturbation while $\tau$ must enforce specific output:
\begin{equation}
|\delta^*| \ll |\tau|
\end{equation}
\end{proof}

\begin{lemma}[High-dimensional Uniform Distribution]
The variance of UAP in high-dimensional space satisfies:
\begin{equation}
|\delta^*| \leq \min{\frac{threshold_{shift}}{\lambda_t}, \frac{\epsilon_{detect}}{\mathbb{E}{\epsilon}[|\nabla_xM\theta(\epsilon)|]}}
\end{equation}
where $d$ is the input dimension.
\end{lemma}
\begin{proof}
In a d-dimensional space, for each dimension i:
\begin{equation}
Var(\delta^_i) \approx \frac{|\delta^|^2}{d}
\end{equation}
The total variance is bounded by:
\begin{equation}
\sum_{i=1}^d Var(\delta^_i) \leq |\delta^|^2
\end{equation}
This uniform distribution property ensures no single dimension contains a detectable signal.
\end{proof}

\subsubsection{Magnitude-Effectiveness Trade-off Analysis}
\begin{theorem}[Computational Bounds]
The bounds $\epsilon_{\text{min}}$ and $\epsilon_{\text{detect}}$ can be computed as:
\begin{equation}
    \epsilon_{\text{min}} = \max\{\frac{\alpha}{\|\nabla_xM_\theta(x)\|}, \frac{\text{dist}(f(x), y_t)}{L}\}
\end{equation}
\begin{equation}
    \epsilon_{\text{detect}} = \min\{\frac{\text{threshold}}{\lambda_{\max}(H)}, \frac{\text{threshold}_{\text{shift}}}{\sqrt{d}}\}
\end{equation}
where:
\begin{itemize}
    \item $L$ is the model's Lipschitz constant
    \item $\lambda_{\max}(H)$ is the maximum eigenvalue of the Hessian
    \item $d$ is the input dimension
\end{itemize}

These bounds relate to model parameters through:
\begin{equation}
    \text{threshold} = O(\frac{1}{\sqrt{d}})
\end{equation}
\begin{equation}
    L = O(\prod_{i=1}^T \sqrt{\bar{\alpha}_i})
\end{equation}
ensuring practical feasibility in high dimensions.
\end{theorem}

% \subsubsection{Model Sensitivity Analysis}
% The effectiveness of UAP depends on model sensitivity:
% \begin{theorem}[Sensitivity Bounds]
% For diffusion model $M_\theta$:
% \begin{equation}
% |M_\theta(x + \delta^) - M_\theta(x)| \leq L|\delta^| + \beta|\delta^*|^2
% \end{equation}
% where:
% \begin{itemize}
% \item $L$ is the local Lipschitz constant
% \item $\beta$ captures second-order effects
% \end{itemize}
% This bound ensures that small UAPs remain effective while evading detection.
% \end{theorem}

% \begin{proposition}[Lipschitz Constant Computation]
% For a diffusion model $M_\theta$, the Lipschitz constant L and second-order coefficient β are computed as:
% \begin{equation}
%     L = \prod_{i=1}^n \|W_i\|
% \end{equation}
% \begin{equation}
%     \beta = \frac{L^2}{2\min_{x}\sigma_{\min}(H(x))}
% \end{equation}

% These bounds ensure UAP effectiveness through:
% \begin{enumerate}
%     \item Small perturbation effectiveness: $L\|\delta^*\| \geq \alpha$ (attack success)
%     \item Detection evasion: $L\|\delta^*\| + \beta\|\delta^*\|^2 < \epsilon_{detect}$
% \end{enumerate}
% \end{proposition}

\subsubsection{Theoretical Bounds}
We can establish sufficient conditions for UAP escape:

\begin{theorem}[UAP Escape Sufficient Condition]
A UAP $\delta$ can escape Elijah's removal if:
\begin{equation}
|\delta| \leq \min \left(\frac{threshold_{shift}}{\lambda_t}, \frac{\epsilon_{detect}}{\mathbb{E}_{\epsilon}[|\nabla_x M_{\theta}(\epsilon)|]} \right)
\end{equation}
\end{theorem}

\begin{proof}
The proof follows from two steps:
\begin{enumerate}
\item For distribution shift: $\lambda_t |\delta| \leq threshold_{shift}$
\item For detection evasion: $|\delta| \mathbb{E}_{\epsilon}[|\nabla_x M_{\theta}(\epsilon)|] \leq \epsilon_{detect}$
\end{enumerate}
Taking the minimum ensures both conditions are satisfied.
\end{proof}

\begin{theorem}[Extended UAP Escape Conditions]
Under the following model-specific assumptions:
\begin{enumerate}
    \item The diffusion model $M_\theta$ follows schedule $\beta_t$
    \item The noise level satisfies $\sum_{t=1}^T \beta_t < B$
    \item The model maintains Lipschitz continuity with constant L
\end{enumerate}

The UAP escape conditions can be refined as:
\begin{equation}
    \|\delta^*\| \leq \min\{\frac{\text{threshold}_{\text{shift}}}{\sqrt{\sum_{t=1}^T \beta_t}}, \frac{\epsilon_{\text{detect}}}{L}\}
\end{equation}
\end{theorem}

\begin{proof}[Complete Proof of Extended Escape Conditions]
The proof consists of three main parts:

1) First, consider the distribution shift condition:
\begin{enumerate}
    \item At each timestep t, the shift is bounded by:
    \begin{equation}
        \|\Delta_{shift}(x_t)\| \leq \lambda_t\|\delta^*\|
    \end{equation}
    \item The cumulative effect across timesteps:
    \begin{equation}
        \sum_{t=1}^T \|\Delta_{shift}(x_t)\| \leq \|\delta^*\|\sqrt{\sum_{t=1}^T \beta_t}
    \end{equation}
\end{enumerate}

2) For the detection evasion condition:
\begin{equation}
    \|M_\theta(x + \delta^*) - M_\theta(x)\| \leq L\|\delta^*\|
\end{equation}

3) Considering model-specific factors:
\begin{itemize}
    \item Effect of noise schedule: $\beta_t$ affects perturbation propagation
    \item Lipschitz constant L depends on model architecture
    \item Detection threshold $\epsilon_{\text{detect}}$ varies with model complexity
\end{itemize}

Taking the minimum of these bounds ensures both conditions are satisfied while accounting for model-specific characteristics.
\end{proof}

\subsubsection{Practical Implementation Considerations}
\begin{theorem}[Practical Feasibility]
The computed bounds are practically achievable when:
\begin{equation}
    \frac{\alpha}{L} \leq \min\{\frac{\text{threshold}_{\text{shift}}}{\sqrt{\sum_{t=1}^T \beta_t}}, \frac{\epsilon_{\text{detect}}}{L}\}
\end{equation}
where $\alpha$ is the minimum required attack success rate.
\end{theorem}

\begin{proof}
This follows from:
\begin{enumerate}
    \item Attack effectiveness requires: $\|\delta^*\| \geq \frac{\alpha}{L}$
    \item Detection evasion requires: $\|\delta^*\| \leq \min\{\frac{\text{threshold}_{\text{shift}}}{\sqrt{\sum_{t=1}^T \beta_t}}, \frac{\epsilon_{\text{detect}}}{L}\}$
    \item These conditions are compatible when the inequality holds
\end{enumerate}
\end{proof}

\begin{tikzpicture}[
    declare function={
        gauss(\x,\m,\s)=1/(2*3.14159*\s*\s)*exp(-(\x-\m)*(\x-\m)/(2*\s*\s));
    }
]
    % 坐标轴
    \draw[->] (-0.5,0) -- (8,0) node[right] {$x$};
    \draw[->] (0,-0.1) -- (0,1.2) node[above] {Probability Density};
    
    % Original Diffusion Distribution at time t
    \draw[thick, blue] plot[domain=0:8,samples=100] 
        (\x,{2*gauss(\x,3,(1-0.7))}) 
        node[pos=0.85, above] {$q(x_t|x_0)$};
    
    % UAP-perturbed Distribution 
    \draw[thick, red, dashed] plot[domain=0:8,samples=100] 
        (\x,{2*gauss(\x,3+0.3*sqrt(0.7),(1-0.7))}) 
        node[pos=0.7, above] {$q(x_t'|x_0)$};
    
    % Traditional Trigger Distribution
    \draw[thick, green!70!black, dotted] plot[domain=0:8,samples=100] 
        (\x,{2*gauss(\x,3+(1-sqrt(0.7))*2,(1-0.7))}) 
        node[pos=0.8, below] {$q(x_t^b|x_0)$};
    
    % Reference lines
    \draw[dashed, gray] (3,0) -- (3,1);
    \draw[dashed, gray] (3.3,0) -- (3.3,1);
    \draw[dashed, gray] (4.5,0) -- (4.5,1);
    
    % Labels
    \node[below] at (3,0) {$\sqrt{\bar{\alpha}_t}x_0$};
    \node[below] at (3.3,0) {$\sqrt{\bar{\alpha}_t}(x_0+\delta^*)$};
    \node[below] at (4.5,0) {$\sqrt{\bar{\alpha}_t}x_0+(1-\sqrt{\bar{\alpha}_t})r$};
    
    % Shift Annotations
    \draw[<->, red] (3.1,0.75) -- (3.5,0.75) 
        node[midway, above, red] {$\sqrt{\bar{\alpha}_t}\|\delta^*\|$};
    \draw[<->, green!70!black] (3.5,0.55) -- (4.7,0.55) 
        node[midway, above, green!70!black] {$(1-\sqrt{\bar{\alpha}_t})\|r\|$};
\end{tikzpicture}

\subsubsection{Implications}

\paragraph{Detection Evasion}
UAP can evade detection because:
\begin{equation}
    \sqrt{\bar{\alpha}_t}\|\delta^*\| < \epsilon_{detect} \ll (1-\sqrt{\bar{\alpha}_t})\|r\|
\end{equation}
where $\epsilon_{detect}$ is the detection threshold.

\subsubsection{Sensitivity}

\begin{tikzpicture}[
    declare function={
        gauss(\x,\m,\s)=1/(2*3.14159*\s*\s)*exp(-(\x-\m)*(\x-\m)/(2*\s*\s));
    }
]
    % 坐标轴
    \draw[->] (-0.5,0) -- (8,0) node[right] {$x$};
    \draw[->] (0,-0.1) -- (0,1.2) node[above] {Probability Density};
    
    % 原始分布（蓝色实线）
    \draw[thick, blue] plot[domain=0:8,samples=100] (\x,{2*gauss(\x,3,0.8)}) 
        node[pos=0.85, above] {Clean Distribution};
    
    % GUAP扰动后的分布（红色虚线，轻微偏移）
    \draw[thick, red, dashed] plot[domain=0:8,samples=100] (\x,{2*gauss(\x,3.3,0.8)}) 
        node[pos=0.7, above] {GUAP-perturbed};
    
    % 传统触发器的分布（绿色点线，大幅偏移）
    \draw[thick, green!70!black, dotted] plot[domain=0:8,samples=100] (\x,{2*gauss(\x,5,0.8)}) 
        node[pos=0.8, below] {Traditional Trigger};
    
    % 垂直界限线
    \draw[dashed, gray] (3,0) -- (3,1);
    \draw[dashed, gray] (3.3,0) -- (3.3,1);
    \draw[dashed, gray] (5,0) -- (5,1);
    
    % 标签
    \node[below] at (3,0) {$\mu_c$};
    \node[below] at (3.3,0) {$\mu_c + \delta^*$};
    \node[below] at (5,0) {$\mu_c + \tau$};
    
    % 说明箭头和文本
    \draw[<->, red] (3.1,0.75) -- (3.5,0.75) 
        node[midway, above, red] {$\epsilon_{detect}$};
    \draw[<->, green!70!black] (3.5,0.55) -- (5,0.55) 
        node[midway, above, green!70!black] {$\epsilon_{detect}$};
    
    % 添加检测阈值区域
    \fill[yellow!20, opacity=0.3] (2.8,0) rectangle (3.5,1.2);
    \node[rotate=90] at (2.7,0.6) {Detection Threshold};

\end{tikzpicture}

\begin{tikzpicture}[
    declare function={
        gauss(\x,\m,\s)=1/(2*3.14159*\s*\s)*exp(-(\x-\m)*(\x-\m)/(2*\s*\s));
    }
]
    % 坐标轴
    \draw[->] (-0.5,0) -- (8,0) node[right] {$x$};
    \draw[->] (0,-0.1) -- (0,1.2) node[above] {Probability Density};
    
    % Original Diffusion Distribution at time t
    \draw[thick, blue] plot[domain=0:8,samples=100] 
        (\x,{2*gauss(\x,3,(1-0.7))}) 
        node[pos=0.85, above] {$q(x_t|x_0)$};
    
    % UAP-perturbed Distribution (small shift proportional to √(ᾱt))
    \draw[thick, red, dashed] plot[domain=0:8,samples=100] 
        (\x,{2*gauss(\x,3+0.3*sqrt(0.7),(1-0.7))}) 
        node[pos=0.7, above] {$q(x_t'|x_0)$};
    
    % Traditional Trigger Distribution (large shift (1-√(ᾱt)))
    \draw[thick, green!70!black, dotted] plot[domain=0:8,samples=100] 
        (\x,{2*gauss(\x,3+(1-sqrt(0.7))*2,(1-0.7))}) 
        node[pos=0.8, below] {$q(x_t^b|x_0)$};
    
    % Reference lines
    \draw[dashed, gray] (3,0) -- (3,1);
    \draw[dashed, gray] (3.3,0) -- (3.3,1);
    \draw[dashed, gray] (4.5,0) -- (4.5,1);
    
    % Labels
    \node[below] at (3,0) {$\sqrt{\bar{\alpha_t}}x_0$};
    \node[below] at (3.3,0) {$\sqrt{\bar{\alpha_t}}(x_0+\delta^*)$};
    \node[below] at (4.5,0) {$\sqrt{\bar{\alpha_t}}x_0+(1-\sqrt{\bar{\alpha_t}})r$};
    
    % Shift Annotations
    \draw[<->, red] (3.1,0.75) -- (3.5,0.75) 
        node[midway, above, red] {$\sqrt{\bar{\alpha_t}}\|\delta^*\|$};
    \draw[<->, green!70!black] (3.5,0.55) -- (4.7,0.55) 
        node[midway, above, green!70!black] {$(1-\sqrt{\bar{\alpha_t}})\|r\|$};
    
    % Time annotation
    \node[above] at (4,1.1) {Timestep $t$};
\end{tikzpicture}

\begin{tikzpicture}[
    declare function={
        gauss(\x,\m,\s)=1/(2*3.14159*\s*\s)*exp(-(\x-\m)*(\x-\m)/(2*\s*\s));
    }
]
    % Traditional Trigger Distribution Shift (Top)
    \begin{scope}[yshift=2cm]
        % Axes
        \draw[->] (-0.5,0) -- (8,0) node[right] {$x$};
        \draw[->] (0,-0.1) -- (0,1.2);
        
        % Original Gaussian
        \draw[thick, green!70!black] plot[domain=0:8,samples=100] 
            (\x,{2*gauss(\x,3,0.8)});
        
        % Shifted Gaussian
        \draw[thick, red, dashed] plot[domain=0:8,samples=100] 
            (\x,{2*gauss(\x,5,0.8)});
        
        % Reference lines
        \draw[dotted] (3,0) -- (3,1);
        \draw[dotted] (5,0) -- (5,1);
        
        % Labels
        \node[above] at (4,1.1) {Traditional Trigger: Distribution Shift};
        \node[below] at (3,0) {$\mu_c^t$};
        \node[below] at (5,0) {$\mu_b^t=\mu_c^t+\lambda^t\tau$};
    \end{scope}
    
    % UAP Effect in Diffusion (Bottom)
    \begin{scope}[yshift=-2cm]
        % Axes
        \draw[->] (-0.5,0) -- (8,0) node[right] {$x$};
        \draw[->] (0,-0.1) -- (0,1.2);
        
        % Original Gaussian
        \draw[thick, green!70!black] plot[domain=0:8,samples=100] 
            (\x,{2*gauss(\x,4,0.8)});
        
        % UAP affected Gaussian (same mean, different variance)
        \draw[thick, blue, dashed] plot[domain=0:8,samples=100] 
            (\x,{2*gauss(\x,4,0.9)});
        
        % Reference lines
        \draw[dotted] (4,0) -- (4,1);
        
        % Labels
        \node[above] at (4,1.1) {UAP in Diffusion: Parameter Change};
        \node[below] at (4,0) {$\mu^t$};
    \end{scope}

    % Additional explanatory text
    \node[right] at (8,2) {Clear shift in distribution center};
    \node[right] at (8,-2) {Changes in distribution parameters};
\end{tikzpicture}

\begin{tikzpicture}[
    declare function={
        gauss(\x,\m,\s)=1/(2*3.14159*\s*\s)*exp(-(\x-\m)*(\x-\m)/(2*\s*\s));
    }
]
    % t很小时的分布 (t→0)
    \begin{scope}[yshift=4cm]
        \draw[->] (-0.5,0) -- (8,0) node[right] {$x$};
        \draw[->] (0,-0.1) -- (0,1.2);
        
        % Original distribution
        \draw[thick, blue] plot[domain=0:8,samples=100] 
            (\x,{2*gauss(\x,3,0.5)}) 
            node[pos=0.85, above] {$q(x_t|x_0)$};
        
        % UAP-shifted
        \draw[thick, red, dashed] plot[domain=0:8,samples=100] 
            (\x,{2*gauss(\x,3.4,0.5)})
            node[pos=0.7, above] {UAP: $q(x_t'|x_0)$};
            
        % Traditional trigger (small shift at early stage)
        \draw[thick, green!70!black, dotted] plot[domain=0:8,samples=100] 
            (\x,{2*gauss(\x,3.2,0.5)})
            node[pos=0.9, below] {Trad: $q(x_t^b|x_0)$};
            
        \node[above] at (4,1.1) {$t \to 0$ (Early Stage)};
        
        % 标注shifts
        \draw[<->, red] (3,0.9) -- (3.4,0.9) 
            node[midway, above] {$\sqrt{\bar{\alpha}_t}\delta^*$ (large)};
        \draw[<->, green!70!black] (3,0.7) -- (3.2,0.7) 
            node[midway, above] {$(1-\sqrt{\bar{\alpha}_t})r$ (small)};
    \end{scope}
    
    % t中等时的分布
    \begin{scope}[yshift=0cm]
        \draw[->] (-0.5,0) -- (8,0) node[right] {$x$};
        \draw[->] (0,-0.1) -- (0,1.2);
        
        % Original
        \draw[thick, blue] plot[domain=0:8,samples=100] 
            (\x,{2*gauss(\x,3,0.5)});
        
        % UAP-shifted (medium shift)
        \draw[thick, red, dashed] plot[domain=0:8,samples=100] 
            (\x,{2*gauss(\x,3.2,0.5)});
            
        % Traditional trigger (medium shift)
        \draw[thick, green!70!black, dotted] plot[domain=0:8,samples=100] 
            (\x,{2*gauss(\x,3.8,0.5)});
            
        \node[above] at (4,1.1) {$t = T/2$ (Middle Stage)};
        
        % 标注shifts
        \draw[<->, red] (3,0.9) -- (3.2,0.9) 
            node[midway, above] {$\sqrt{\bar{\alpha}_t}\delta^*$ (medium)};
        \draw[<->, green!70!black] (3,0.7) -- (3.8,0.7) 
            node[midway, above] {$(1-\sqrt{\bar{\alpha}_t})r$ (medium)};
    \end{scope}
    
    % t很大时的分布 (t→T)
    \begin{scope}[yshift=-4cm]
        \draw[->] (-0.5,0) -- (8,0) node[right] {$x$};
        \draw[->] (0,-0.1) -- (0,1.2);
        
        % Original
        \draw[thick, blue] plot[domain=0:8,samples=100] 
            (\x,{2*gauss(\x,3,0.5)});
        
        % UAP-shifted (tiny shift)
        \draw[thick, red, dashed] plot[domain=0:8,samples=100] 
            (\x,{2*gauss(\x,3.05,0.5)});
            
        % Traditional trigger (large shift)
        \draw[thick, green!70!black, dotted] plot[domain=0:8,samples=100] 
            (\x,{2*gauss(\x,4.5,0.5)});
            
        \node[above] at (4,1.1) {$t \to T$ (Late Stage)};
        
        % 标注shifts
        \draw[<->, red] (3,0.9) -- (3.05,0.9) 
            node[midway, above] {$\sqrt{\bar{\alpha}_t}\delta^*$ (small)};
        \draw[<->, green!70!black] (3,0.7) -- (4.5,0.7) 
            node[midway, above] {$(1-\sqrt{\bar{\alpha}_t})r$ (large)};
    \end{scope}
    
    % 添加说明
    \node[right] at (8,-2) {Key Properties:};
    \node[right] at (8,-2.5) {1. All distributions maintain same variance $(1-\bar{\alpha}_t)I$};
    \node[right] at (8,-3) {2. UAP shift $\sqrt{\bar{\alpha}_t}\delta^*$ decreases with $t$};
    \node[right] at (8,-3.5) {3. Traditional shift $(1-\sqrt{\bar{\alpha}_t})r$ increases with $t$};
\end{tikzpicture}

\begin{tikzpicture}
    % 坐标轴
    \draw[->] (0,0) -- (8,0) node[right] {$t$};
    \draw[->] (0,-1) -- (0,4) node[above] {Impact};
    
    % Generation importance curve
    \draw[blue, thick] plot[domain=0:8,smooth] 
        coordinates {(0,3) (2,2.5) (4,1.5) (6,0.5) (8,0.2)}
        node[right] {Generation Importance};
    
    % UAP shift curve
    \draw[red, thick, dashed] plot[domain=0:8,smooth] 
        coordinates {(0,3.5) (2,2) (4,1) (6,0.3) (8,0.1)}
        node[right] {UAP Shift};
    
    % Traditional trigger shift curve
    \draw[green!70!black, thick, dotted] plot[domain=0:8,smooth] 
        coordinates {(0,0.2) (2,0.8) (4,1.8) (6,2.8) (8,3.5)}
        node[right] {Traditional Shift};
    
    % Effective impact regions
    \fill[red!20, opacity=0.3] (0,0) -- plot[domain=0:4,smooth] 
        coordinates {(0,3.5) (1,2.8) (2,2) (3,1.4) (4,1)} -- (4,0) -- cycle;
    \node[red] at (1,1) {Critical Impact Region};
    
    % Time annotations
    \node[below] at (0,-0.2) {$t=0$};
    \node[below] at (8,-0.2) {$t=T$};
    
    % Legend
    \node[right] at (8,3.5) {High};
    \node[right] at (8,0) {Low};
\end{tikzpicture}
